# Supplementary material for: A GPU-accelerated Cartesian grid method for PDEs on irregular domain
Source: arXiv:2404.15249 source file (2024-04-23)
Supplement: Supplementary file 1 [file Appendix.tex]

\section{Appendix}
\subsection{KFBI method for Neumann boundary condition}\label{appen::neumann::condition}
The Dirichlet BVP has been introduced in $\ref{introduce_kfbi}$ for the sake of clarity. In this section, the modified Helmholtz equation $\eqref{one_GPU:modified_helmholtz}$ subject to Neumann boundary condition is considered as:
\begin{equation}
    \partial_{\mathbf{n}}u(\mathbf{x}) = g_{N}(\mathbf{x}). \label{Neumann}
\end{equation}
Similarly to the Dirichlet boundary condition, the single layer potential is defined as
\begin{equation}
    (S\psi)(\mathbf{x}) := \int_{\Gamma} G(\mathbf{y}, \mathbf{x}) \psi(\mathbf{y}) d s_{\mathbf{y}} ~\text { for } ~\mathbf{x} \in \Omega \cup \Omega^{c}. \label{single}
\end{equation}

Owing to detonations defined above, the BIE $\eqref{one_GPU:modified_helmholtz}$ and $\eqref{Neumann}$ also can be reformulated as a Fredholm boundary integral equation of the second kind\cite{kress1989linear,hsiao2008boundary}, which follows
\begin{equation}
    \frac{1}{2}\psi(\mathbf{x}) -\partial_{\mathbf{n}} (S\psi)(\mathbf{x}) + \partial_{\mathbf{n}} (Yf)(\mathbf{x}) = g_{N}(\mathbf{x}).
    \label{fredholm:neumann}
\end{equation}
The solution $u(\mathbf{x})$ to Neumann BVP $\eqref{one_GPU:modified_helmholtz}$ and $\eqref{Neumann}$ is given by 
\begin{equation}
    u(\mathbf{x}) = (Yf)(\mathbf{x}) - (S\psi)(\mathbf{x}), \quad x \in \Omega.
\end{equation}
Numerically, the boundary integral equation $\eqref{fredholm:neumann}$ can be solved by simply fixed point iteration: given the artificial initial guess $\psi_{0}(\mathbf{x})$, for $k \in \left\{0, 1, 2, 3, \cdots \right\}$, do as follows:
\begin{align}
    \partial_{\mathbf{n}} u_{k}^{+}(\mathbf{x}_{m}) = \frac{1}{2}\psi(\mathbf{x}_{m}) - \partial_{\mathbf{n}}(S\psi)(\mathbf{x}_{m}), & \quad \mathbf{x}_{m} \in \Gamma,\label{neumann:richardson1} \\
    \psi_{k+1}(\mathbf{x}_{m}) = \psi_{k}(\mathbf{x}_{m}) + \gamma[\hat{g}_{N}(\mathbf{x}_{m}) - \partial_{\mathbf{n}} u_{k}^{+}(\mathbf{x}_{m})], & \quad \mathbf{x}_{m} \in \Gamma.\label{neumann:richardson2}
\end{align}
Here, $\hat{g}_{N}(\mathbf{x}_{m}) = g_{N}(\mathbf{x}_{m})-\partial_{\mathbf{n}}(Yf)(\mathbf{x}_{m}),\text{ for } \mathbf{x}_{m} \in \Gamma$. $\mathbf{x}_{m}$ is the control node located on interface. Suppose $w(\mathbf{x})$ is an arbitrary piecewise smooth function with derivative  discontinuities on the interface $\Gamma$: 
\begin{equation}
    \partial_{\mathbf{n}} w^{+}(\mathbf{x}) = \lim_{z \longrightarrow x, z \in \Omega} \partial _{\mathbf{n}} w(\mathbf{z}),
\end{equation}
$\partial_{\mathbf{n}} w^{-}(\mathbf{x})$ can be defined in the same way. 

As for Neumann BVP, the single layer boundary integral $\eqref{fredholm:neumann}$  $u(\mathbf{x}{x})$ can be considered as a solution to the following interface problem:
\begin{equation}
\begin{array}{ll}
\Delta v(\mathbf{x})-\kappa v(\mathbf{x})=0, &\text { for } \mathbf{x} \in \Omega \cup \Omega^{c},\\
{[v(\mathbf{x})]=0}, & \text { for } \mathbf{x} \in \Gamma,\\
{\left[\partial_{\mathbf{n}} v(\mathbf{x})\right]=\psi(\mathbf{x})}, & \text { for } \mathbf{x} \in \Gamma,\\
v(\mathbf{x})=0. & \text { for } \mathbf{x} \in \partial \mathcal{B}.
\end{array}
\label{single:interface}
\end{equation}

The KFBI method is characterized by the transformation of the integral  $\eqref{single}$  into the solution of the interface problem $\eqref{single:interface}$. In contrast to the Dirichlet problem, the Neumann problem also goes through the three steps of correction, fast solving interface problem, and boundary interpolation. The difference is that the Neumann problem requires interpolation of normal derivatives in $\eqref{neumann:richardson2}$ instead of boundary values in $\eqref{one_GPU:richardson2}$. In addition to this, the main steps of GMRES iteration are the same for both boundary condition except $\mathcal{K}_{N}(\varphi)(\mathbf{x})$ is replaced by 
\begin{equation}
    \mathcal{K}_{N}(\psi)(\mathbf{x}) := \frac{1}{2}\psi(\mathbf{x}) - \partial_{\mathbf{n}}(S\psi)(\mathbf{x}), \quad \mathbf{x} \in \Gamma.
\end{equation}
